# Supplementary material for: The merger of spinning, accreting supermassive black hole binaries
Source: arXiv:2509.10319 ancillary file (2025-12-03)
Supplement: Supplementary file 1 [file PRL_SupplementalMaterial.pdf]

# The merger of spinning, accreting supermassive black hole binaries

## Supplemental Material

Lorenzo Ennoggi 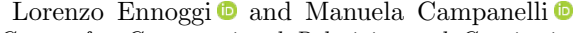 and Manuela Campanelli 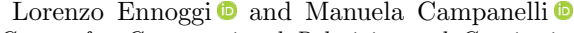

*Center for Computational Relativity and Gravitation,*

*Rochester Institute of Technology & School of Physics and Astronomy, Rochester, New York 14623, USA*

Julian Krolik 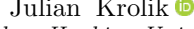

*Physics and Astronomy Department, Johns Hopkins University, Baltimore, Maryland 21218, USA*

Scott C. Noble 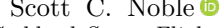

*Gravitational Astrophysics Lab, NASA Goddard Space Flight Center, Greenbelt, Maryland 20771, USA*

Yosef Zlochower 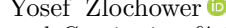

*Center for Computational Relativity and Gravitation & School of Mathematics and Statistics,*

*Rochester Institute of Technology, Rochester, New York 14623, USA*

Maria Chiara de Simone 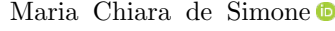

*Center for Computational Relativity and Gravitation,*

*Rochester Institute of Technology & School of Physics and Astronomy, Rochester, New York 14623, USA*

(Dated: September 12, 2025)

Figure 1 shows scatter plots of the photon and Poynting luminosities,  $L_{\text{photons}}$  and  $L_{\text{Poynting}}$ , respectively, vs. the gas mass  $M_{\text{gas}}$  within  $r \leq 15 M$  of the center of mass of the system and the total mass accretion rate  $\dot{M}$  onto the black holes from  $t \simeq 103000 M$  to the end of the simulation. In all of these plots, and especially in the  $L_{\text{photons}}$  vs.  $M_{\text{gas}}$  (top-left panel) and  $L_{\text{Poynting}}$  vs.  $M_{\text{gas}}$  (bottom-left panel) ones, we can clearly distinguish three periods of time: the early inspiral ( $103000 M \lesssim t \lesssim 108000 M$ , blue data), the late inspiral ( $108000 M \lesssim t \leq t_{\text{merger}}$  with  $t_{\text{merger}} \simeq 115000 M$ , red data), and the postmerger ( $t > t_{\text{merger}}$ , green data).

The linear least-squares fit to the data in log space in each time period is shown as a straight line colored to match its corresponding data set; the slope of each line represents the exponent  $\alpha$  in the relationship  $f(x) = x^\alpha$ , where  $f$  is either  $L_{\text{photons}}$  or  $L_{\text{Poynting}}$  and  $x$  is either  $M_{\text{gas}}$  or  $\dot{M}$ . Table I lists the coefficients  $\alpha$  and the Pearson correlation coefficients (“Pearson  $r$ ”) for all the linear fits shown in Figure 1. As already evident from visual inspection of Figure 1, the strongest correlations occur during the early inspiral part of the simulation and link  $M_{\text{gas}}$  to the two luminosities,  $L_{\text{photons}}$  and  $L_{\text{Poynting}}$ . For the first relation we have  $\alpha = 0.3247 \pm 0.0003$  with Pearson  $r \simeq 0.83$ , while the second one gives  $\alpha = 0.3141 \pm 0.0003$  with Pearson  $r \simeq 0.82$ .

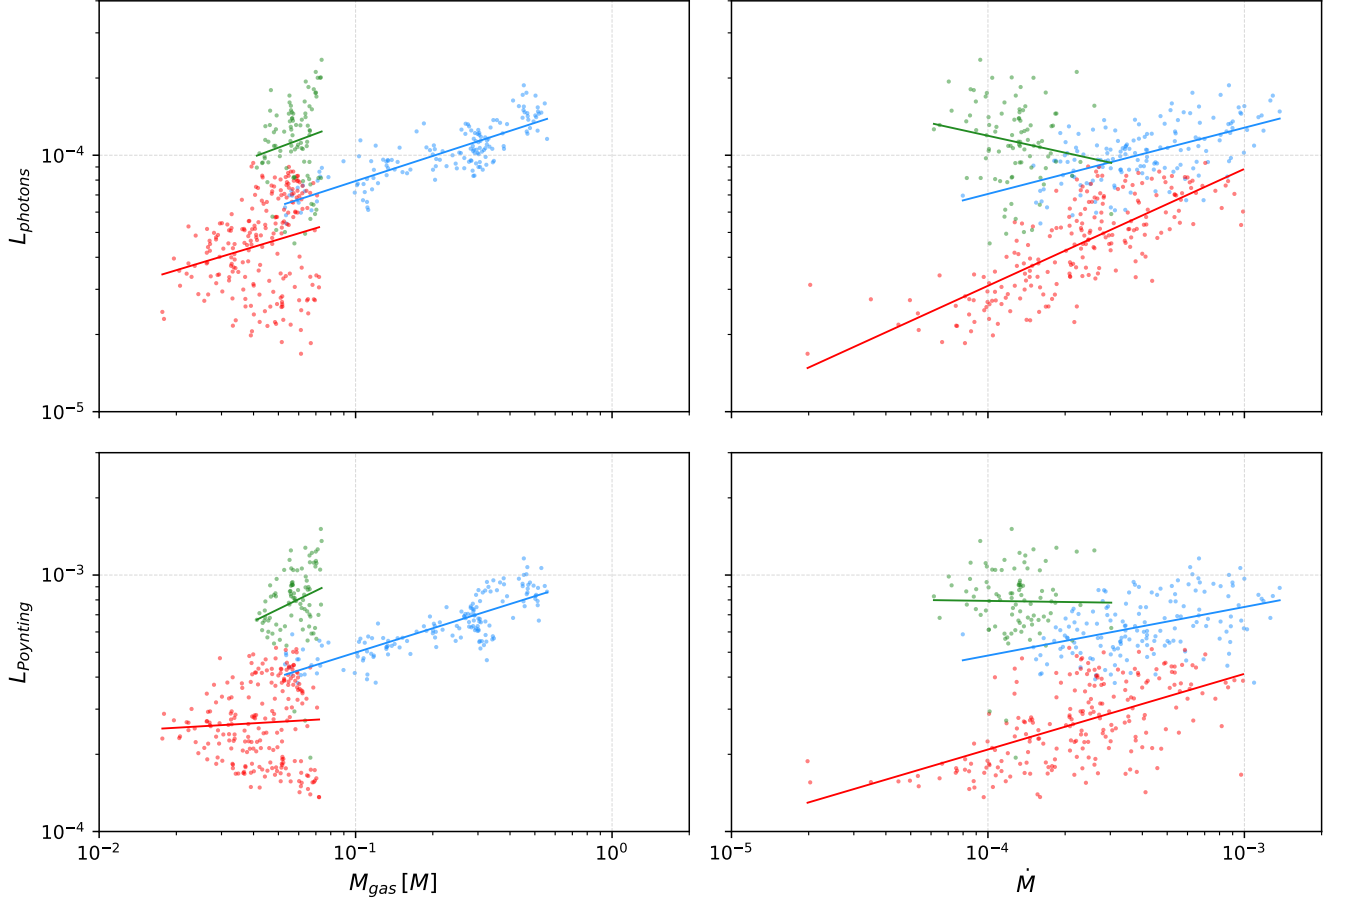

**Figure 1:** Scatter plots of  $L_{\text{photons}}$  and  $L_{\text{Poynting}}$  vs.  $M_{\text{gas}}$  and  $\dot{M}$  during the early inspiral (blue, times  $103000 M \lesssim t \lesssim 108000 M$ ), late inspiral (red, times  $108000 M \lesssim t \leq t_{\text{merger}}$ ), and postmerger (green, times  $t > t_{\text{merger}}$ ) stages of the simulation. For each subplot, the solid lines represent the best fit to the data in each of the three time ranges.

|                  | Early inspiral (blue) | Late inspiral (red) | Postmerger (green) |
|------------------|-----------------------|---------------------|--------------------|
| $\alpha$ (slope) | $0.3247 \pm 0.0003$   | $0.301 \pm 0.008$   | $0.37 \pm 0.06$    |
| Pearson $r$      | 0.83                  | 0.23                | 0.16               |

(a)  $L_{\text{photons}}$  vs.  $\dot{M}_{\text{gas}}$  (top-left panel of Figure 1)

|                  | Early inspiral (blue) | Late inspiral (red) | Postmerger (green) |
|------------------|-----------------------|---------------------|--------------------|
| $\alpha$ (slope) | $0.2583 \pm 0.0009$   | $0.4558 \pm 0.0007$ | $-0.22 \pm 0.02$   |
| Pearson $r$      | 0.57                  | 0.76                | -0.17              |

(b)  $L_{\text{photons}}$  vs.  $\dot{M}$  (top-right panel of Figure 1)

|                  | Early inspiral (blue) | Late inspiral (red) | Postmerger (green) |
|------------------|-----------------------|---------------------|--------------------|
| $\alpha$ (slope) | $0.3141 \pm 0.0003$   | $0.577 \pm 0.006$   | $0.49 \pm 0.04$    |
| Pearson $r$      | 0.82                  | 0.50                | 0.24               |

(c)  $L_{\text{Poynting}}$  vs.  $\dot{M}_{\text{gas}}$  (bottom-left panel of Figure 1)

|                  | Early inspiral (blue) | Late inspiral (red) | Postmerger (green) |
|------------------|-----------------------|---------------------|--------------------|
| $\alpha$ (slope) | $0.189 \pm 0.001$     | $0.2950 \pm 0.0009$ | $-0.01 \pm 0.01$   |
| Pearson $r$      | 0.42                  | 0.56                | -0.12              |

(d)  $L_{\text{Poynting}}$  vs.  $\dot{M}$  (bottom-right panel of Figure 1)

**Table I:** Linear least-squares fit parameters for all the subplots in Figure 1 and all three time periods (early inspiral, late inspiral, postmerger) in each subplot. The colors “blue”, “red”, and “green” match the convention used in Figure 1 to indicate each of these time periods.
